# Supplementary material for: Enhanced configurational entropy in high-density nanoconfined bilayer ice
Source: arXiv:1506.04668 source file (2016-02-26)
Supplement: Supplementary file 1 [file supplemental_material.pdf]

arXiv [cond-mat.soft]

Supplemental Material for:
Enhanced configurational entropy in high-density nanoconfined bilayer ice
Fabiano Corsetti, Jon Zubeltzu, Emilio Artacho

## PHASE TRANSITION IN THE $NVE$ AND $NP_{xy}T$ ENSEMBLES

The proposed phase transition between the proton-ordered square tubes phase and the proton-disordered triangular phase is verified by performing calculations both in the $NVE$ and $NP_{xy}T$ ensembles. The results are shown in Fig. S1. For $NVE$ we perform heating and cooling processes (described in the main text), while for $NP_{xy}T$ each point is equilibrated independently for 30 ns, after which statistics are collected for 100 ps. In the $NP_{xy}T$ ensemble the size and shape of the cell in the $xy$ plane are free to change (while the confinement width is fixed to 8 Å in z). Unless specified, calculations are of 294 water molecules.

The difference in entropy between the two phases $\Delta S$ is estimated by calculating $\Delta U/T_c$ for $NVE$ and $\Delta H/T_c$ for $NP_{xy}T$. The same phase transition is observed in both cases. From $NP_{xy}T$, we find a transition temperature $T_c \simeq 272 \pm 2$ K and a change in entropy $\Delta S \simeq 0.72 \pm 0.05$; both are well within the error margins given in the main text for the corresponding values calculated from the $NVE$ heating and cooling curves.

We also verify that finite size effects do not affect our results by performing two simulations at twice the system size (588 molecules) on either side of the transition. As can be seen in Fig. S1, the difference in energy with the standard system size is within the level of the statistical fluctuations.

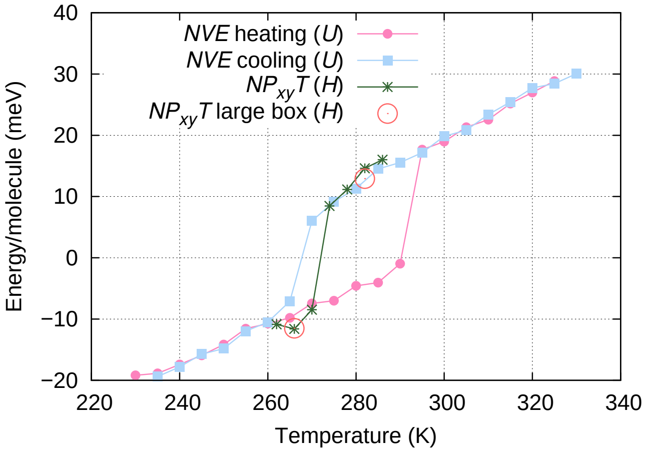


FIG. S1. Comparison of $NVE$ and $NP_{xy}T$ calculations. We plot the internal energy $U$ for $NVE$ and the enthalpy $H$ for $NP_{xy}T$. The reference energy for the two different ensembles is taken to be at the mid-point of the phase transition at $\sim 272$ K. The lateral pressure for $NP_{xy}T$ is fixed at 11.5 GPa Å. All simulations are of 294 molecules, except '$NP_{xy}T$ large box' which are of 588 molecules.

Finally, we note that phase coexistence is observed in some $NVE$ runs close to $T_c$; this is again consistent with a first-order transition. Fig. S2 shows the structure obtained for one such run.

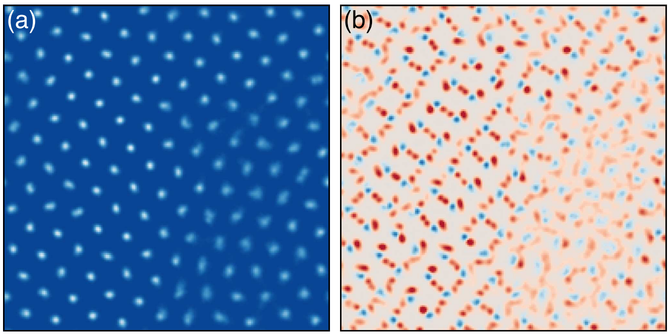


FIG. S2. Example of phase coexistence in an $NVE$ ensemble simulation ($T = 265$ K). (a) Oxygen positions averaged over the entire run; both layers are included. (b) The same system with both the oxygens (in blue) and protons (in red) shown. The proton-ordered square tubes phase can be seen on the top left of the cell, and the proton-disordered triangular phase on the bottom right.

## CONFIGURATIONAL ENTROPY MODEL CALCULATIONS

A Pauling-like estimate of the configurational entropy of triangular bilayer ice can be calculated numerically using the lattice model presented in the main text. We do so as follows: Firstly, the two layers are combined into a single triangular lattice; the configuration of a combined lattice site is therefore given by the configurations of the upper and lower molecules, one of which must be in-plane and the other one out-of-plane ($s = 120 \times 60 = 7200$ possible distinguishable configurations for one combined site). The number of combined lattice sites is $M = N/2$. These are divided into three disjoint sublattices forming a tripartite graph. The number of microstates for the first sublattice is $W_1 = s^{M/3}$. Each site of the second sublattice then has three fixed neighbors belonging to the first sublattice; the number of microstates is $W_2 = \alpha^{M/3}$, where $\alpha$ is the average number of allowed configurations for a lattice site, given three fixed neighbors chosen at random. Finally, each site of the third sublattice has all six neighbors fixed from the other two sublattices; the number of microstates is $W_3 = \beta^{M/3}$, where $\beta$ is the probability for a random choice of six compatible neighboring configurations to produce an allowed configuration at the central lattice site. The total number of microstates for the entire system is $W = W_1 W_2 W_3$. This takes account both of the bond and the proton disorder. We note that $W_2$ can be computed exactly by explicit counting, while $W_3$ is estimated by a Monte Carlo method. Table SI gives the resulting entropy for a number of possible sets of allowed proton configurations.

TABLE SI. Configurational entropy of triangular bilayer ice calculated using different sets of proton configurations (Fig. 5 in the main text). The values of $s$, $\alpha$ and $\beta$ from which $W$ is calculated are also included. The direct estimate from MD is listed at the end for comparison. The first set ($A1$+$A1$*) gives no allowed microstates, as the use of these two configurations on their own requires a honeycomb topology instead of a triangular one to satisfy the ice rules.

| Allowed proton configurations | $s$ | $\alpha$ | $\beta$ | $W$ | $S/N\ (k_B)$ |
|---|---|---|---|---|---|
| $A1$+$A1$* | 72 | 0.4 | 0 | 0 | - |
| $B1$+$B1$*+$B2$+$B2$* | 1152 | 2.5 | $0.004 \pm 0.001$ | $(1.5 \pm 0.1)^N$ | $0.4 \pm 0.1$ |
| $A1$+$A1$*+$B1$+$B1$*+$B2$+$B2$* | 1800 | 4.8 | $0.004 \pm 0.001$ | $(1.8 \pm 0.1)^N$ | $0.6 \pm 0.1$ |
| $A1$+$A1$*+$B1$+$B1$*+$B2$+$B2$*+$B3$*+$C1$* | 3240 | 8.3 | $0.006 \pm 0.001$ | $(2.3 \pm 0.1)^N$ | $0.8 \pm 0.1$ |
| All | 7200 | 17.5 | $0.0266 \pm 0.0005$ | $(3.87 \pm 0.01)^N$ | $1.35 \pm 0.01$ |
| MD | | | | $(2.0 \pm 0.2)^N$ | $0.7 \pm 0.1$ |
